# Supplementary material for: Price Competition with Geometric Brownian motion in Exchange Rate Uncertainty
Source: arXiv:1804.08153 source file (2018-04-22)
Supplement: Supplementary file 1 [file Appendix.tex]

\begin{center}\textbf{APPENDIX: Optimal Capacity Investment, and Pricing across International Markets under Exchange Rate Uncertainty and Duopoly Competition }
\end{center}

\noindent \textbf{Proof of Lemma 4.1}

Proof. In order for the manufacturer to export to the foreign market, $Q^{\ast^{+}}_{lf1}$ must be $>0$. The denominator of equation (4.7) is clearly $>0$, however the numerator of (4.7) must be$\,>0:$ $I\left(\alpha_{lf}+\theta P_g\right)-\beta_{lf}(C_l+r)>0$. From the last inequality, we can get the exchange rate threshold, I$_{z1}$.\\

\noindent \textbf{Proof of Proposition 4.1} 

It is straightforward to observe from (4.16) that $\lambda_{l1}$ must be $>0$ in order for the capacity to be limited (i.e., the capacity constraint is binding). This implies that (4.21) must hold. \\

\noindent \textbf{Proof of Proposition 4.2} 

It is straightforward to observe from (4.16) that $\lambda_{l1}$ must be $>0$ in order for the capacity to be limited (i.e., the capacity constraint is binding). This implies that (4.21) must hold.
\begin{equation*}
\frac{\beta_{lf}(\alpha_{lh}+\beta_{lh}r)}{\beta_{lh}(\alpha_{lf}\text{+}%
\theta
P_g-2K_{l1})}>\frac{\beta_{lf}(\alpha_{lh}-2K_{l1}+\beta_{lh}r)}{\beta_{lh}%
\left(\alpha_{lf}\text{+}\theta P_g\right)},
\end{equation*}

which can be rewritten as 

\begin{equation*}
\frac{(\alpha_{lh}+\beta_{lh}r)}{(\alpha_{lfF}\text{+}\theta
P_g-2K_{l1})}>\frac{(\alpha_{lh}-2K_{l1}+\beta_{lh}r)}{\left(\alpha_{lf}%
\text{+}\theta P_g\right)}.
\end{equation*}

It is clear that from the last argument that
$(\alpha_{lh}+\beta_{lh}r)>(\alpha_{lh}-2K_{l1}+\beta_{lh}r)$ and
$(\alpha_{lf}+\theta P_g-2K_{l1})<\left(\alpha_{lf}+\theta P_g\right)$, this
inequality must hold. \\

\noindent \textbf{Proof of Lemma 4.2} 
Lemma 4.2:$\,$ For any given $K_{l1}$, $I_{h1}>I_{t1}$

Proof. 

\begin{equation*}
\frac{\beta_{lf}(\alpha_{lh}+\beta_{lh}r)}{\beta_{lh}(\alpha_{lf}+\theta
P_g-2K_{l1})}>\frac{\beta_{lf}(C_l+r)}{(\alpha_{lh}+\alpha_{lf}-2K_{l1}-%
\beta_{lh}C_l+\theta P_g)}
\end{equation*}

\begin{equation*}
\frac{(\alpha_{lh}+\beta_{lh}r)}{\beta_{lh}(\alpha_{lf}+\theta
P_g-2K_{l1})}>\frac{\left(C_l+r\right)}{(\alpha_{lh}+\alpha_{lf}-2K_{l1}-%
\beta_{lh}C_l+\theta P_g)}
\end{equation*}

It is clear that $(\alpha_{lh}+\beta_{lh}r)>\left(C_l+r\right)$, so how about
the denominator of the last argument.$\,$For$\,$any$\,$given$\,K_{l1}$,$\,$
$(\alpha_{lh}+\alpha_{lf}-2K_{l1}-\beta_{lh}C_l+\theta
P_g)>\beta_{lh}(\alpha_{lf}+\theta P_g-2K_{l1})$.

Lemma 4.3:$\,$ For any given capacity level, $I_{h1}>I_{z1}$

Proof. 

\begin{equation*}
\frac{\beta_{lf}(\alpha_{lh}+\beta_{lh}r)}{\beta_{lh}(\alpha_{lf}+\theta
P_g-2K_{l1})}>\frac{\beta_{lf}(C_l+r)}{\alpha_{lf}\text{+}\theta P_g}
\end{equation*}

It is clear that $(\alpha_{lh}+\beta_{lh}r)>\left(C_l+r\right)$, so how about
the denominator of the last argument. For any given $K_{l1}$,
$(\alpha_{lf}+\theta P_g)>\beta_{lh}(\alpha_{lf}+\theta
P_g-2K_{l1})$.

Lemma 4.4:$\,I_{z1}>I_{f1}\,$for $K_{l1}>Q^{\ast^{+}}_{lh1}\,$otherwise
$I_{f1}>I_{z1}$

Proof. 

\begin{equation*}
\frac{\beta_{lf}(C_l+r)}{\alpha_{lf}\text{+}\theta
P_g}>\frac{\beta_{lf}(\alpha_{lh}-2K_{l1}+\beta_{lh}r)}{\beta_{lh}\left(%
\alpha_{lf}\text{+}\theta P_g\right)}
\end{equation*}

Simplifying the last argument we get:
$0>\alpha_{lh}-2K_{l1}+\beta_{lh}r.\,$The last inequality indicates that: at
$K_{l1}=Q^{\ast^{+}}_{lh1},\,$we find that $I_{z1}=I_{f1}$, and at
$K_{l1}>Q^{\ast^{+}}_{lh1}$, we get $I_{z1}>I_{f1}$, and at
$K_{l1}<Q^{\ast^{+}}_{lh1}$, we get $I_{f1}>I_{z1}$.

Lemma 4.5: $\,I_{t1}>I_{z1}\,\,$if and only if $K_{l1}>Q^{\ast^{+}}_{lh1}$

Proof. \ if capacity level falls below $Q^{\ast^{+}}_{lh1}$, then $I_{t1}$ is irrelevant because capacity is scarce for both markets. We are interested in the situation where $K_{l1}>Q^{\ast^{+}}_{lh1}$:

\begin{equation*}
\frac{\beta_{lf}(C_l+r)}{(\alpha_{lh}+\alpha_{lf}-2K_{l1}-\beta_{lh}C_l+%
\theta P_g)}>\frac{\beta_{lf}(C_l+r)}{\alpha_{lf}\text{+}\theta P_g}
\end{equation*}

Simplifying the last inequality we get:
$0>\alpha_{lh}+\alpha_{lf}-2K_{l1}-\beta_{lh}C_l$. Therefore, for
$K_{l1}>Q^{\ast^{+}}_{lh1},\,$we get $I_{t1}>I_{z1}$. \\

\noindent \textbf{Proof of Lemma 5.3} 

The firm will export to the foreign market only if $Q^{\ast^{+}}_{lf2}>0$. From (5.6) we know that $4\beta_{lf}\beta_g-\theta^2>0$, since $\beta_{ij}>\theta$. So, we are left with numerator which must be $>0$ which is given in $(5.8)$ \\

\noindent \textbf{Proof of Lemma 5.4} 

Solving equations (5.10) and (5.11) in terms of exchange rate (I). \\

\noindent \textbf{Proof of Lemma 5.5} 

From (5.7) where $Q^{\ast^{+}}_g \leq 0 $ .  \\

\noindent \textbf{Proof of Lemma 5.6} 

Solving for $ C_g\,$when $I_{z2}>I_v $ .  \\

\noindent \textbf{Proof of Lemma 5.7} 

By solving the above equation we can obtain $C_m$ .  \\

\noindent \textbf{Proof of Proposition 5.1} 

We derive $I_{t2}$ via $\lambda_{l2}\geq 0.\,$We derive $K_{t2}$ via
$I_{t2}>0$.  \\

\noindent \textbf{Proof of Proposition 5.2} 

The inequality in (5.24) directly follows from the fact that the manufacturer will sell to the domestic market if $Q^{^{\ast^{-}}}_{lh2}>0$ implying that the numerator in (5.18) must be non-negative. This is satisfied when (5.24) holds. Similarly, $Q^{^{\ast^{-}}}_{lf2}>0$ implies that (5.19) holds. Next we show that $I_{f2}<I_{h2}$. First observe that $I_{f2}<I_{h2}$ implies that

\begin{equation*}
\frac{\beta_{lf}\left(\alpha_{lh}+\beta_{lh}r\right)}{\left(\left(\beta_{lf}%
\beta_g\right)\left(2\alpha_{lf}-4K_{l2}+\theta
C_g\right)+\theta\left(\beta_{lf}\alpha_g+\theta
K_{l2}\right)\right)}>\frac{\left(\alpha_{lh}-2K_{l2}+\beta_{lh}r\right)}{%
\left(\beta_g\left(2\alpha_{lf}+\theta C_g\right)+\theta\alpha_g\right)},
\end{equation*}

which can be rewritten as 

$2\beta_{lf}\beta_g\left(2\alpha_{lh}+2\alpha_{lf}+\theta
C_g\right)+\theta\left(2\beta_{lf}\alpha_g+\alpha_{lh}+\beta_{lh}r%
\right)>2K_{l2}\left(4\beta_{lf}\beta_g+\theta\right)$.

It is clear that the above inequality holds. \\

\noindent \textbf{Proof of Lemma 5.10}
The proof is similar to the proof of Lemma 4.2,  Lemma 4.3, Lemma 4.4, and Lemma 4.5.  \\

Proof of equilibrium results

\begin{equation*}
P^{\ast^{-}}_{lh2}=\frac{I\beta_{lf}\beta_g\left(4\alpha_{lh}+2
\alpha_{lf}-4K_{l2}+\theta
C_g\right) + I\theta\left(\theta\left(\alpha_{lh}+K_{l2}\right)+\beta_{lf}\alpha_g
\right)  }{I\beta_{lh}\left(4\beta_{lf}\beta_g-\theta^2\right)+\beta_{lf}
\left(4\beta_{lf}\beta_g-2\theta^2\right)} +
\end{equation*}
\begin{equation*}
\frac{\beta_{lf}\left(\alpha_{lh}-\beta_{lh}r\right)\left(2\beta_{lf}\beta_g-
\theta^2\right)}{\beta_{lh}\left(I\beta_{lh}\left(4\beta_{lf}\beta_g-\theta^2
\right)+\beta_{lf}\left(4\beta_{lf}\beta_g-2\theta^2\right)\right)}\tag*{$
\left(5.15\right)$}
\end{equation*}

\begin{equation*}
P^{\ast^{-}}_{lf2}=\frac{I\beta_{lh}\left(2\beta_g\alpha_{lf}+\theta\left(
\alpha_g+C_g\beta_g\right)\right) + 2\beta_{lf}\left(\beta_g\left(\alpha_{lh}+2\alpha_{lf}-2K_{l2}+\theta
C_g+\beta_{lh}r\right)+\theta\alpha_g\right)}{I\beta_{lh}\left(4\beta_{lf}\beta_g-
\theta^2\right)+\beta_{lf}\left(4\beta_{lf}\beta_g-2\theta^2\right)}\tag*{$
\left(5.16\right)$}
\end{equation*}

Substituting $P^{\ast^{-}}_{lf2}$ in $P^{\ast^{+}}_g\,$, we get
\begin{equation*}
P^{\ast^{-}}_g=\frac{I\beta_{lh}\left(2\beta_{lf}\left(\alpha_g+\beta_gC_g
\right)+\theta\alpha_{lf}\right) + \beta_{lf}\left(\left(2\beta_{lf}\left(\alpha_g+\beta_gC_g\right)+
\theta\alpha_{lf}\right)+\theta\left(\alpha_{lh}+2\alpha_{lf}-2K_{l2}+
\beta_{lh}r\right)\right)  }{I\beta_{lh}\left(4\beta_{lf}\beta_g-
\theta^2\right)+\beta_{lf}\left(4\beta_{lf}\beta_g-2\theta^2\right)} \tag*{$\left(5.17
\right)$}
\end{equation*}

%\begin{equation*}
%\frac{\beta_{lf}\left(\left(2\beta_{lf}\left(\alpha_g+\beta_gC_g\right)+\theta\alpha_{lf}\right)+\theta\left(\alpha_{lh}+2\alpha_{lf}-2K_{l2}+ \beta_{lh}r\right)\right)}{I\beta_{lh}\left(4\beta_{lf}\beta_g-\theta^2\right)+\beta_{lf}\left(4\beta_{lf}\beta_g-2\theta^2\right)}\tag*{$\left(5.17 \right)$}
%\end{equation*}

Thus, 
\begin{equation*}
Q^{^{\ast^{-}}}_{lh2}=\frac{I\beta_{lh}\left(\left(\beta_{lf}\beta_g\right)
\left(4K_{l2}-2\alpha_{lf}-\theta
C_g\right)-\theta\left(\beta_{lf}\alpha_g+\theta
K_{l2}\right)\right)  + \beta_{lf}\left(\alpha_{lh}+\beta_{lh}r\right)\left(2\beta_{lf}
\beta_2-\theta^2\right)}{I\beta_{lh}\left(4\beta_{lf}\beta_g-\theta^2\right)+
\beta_{lf}\left(4\beta_{lf}\beta_g-2\theta^2\right)}\tag*{$(5.18)$}
\end{equation*}

\begin{equation*}
Q^{^{\ast^{-}}}_{lf2}=\frac{I\beta_{lf}\beta_{lh}\left(\beta_g\left(2
\alpha_{lf}+\theta
C_g\right)+\theta\alpha_g\right)  -  \beta_{lf}\left(\alpha_{lh}-2K_{l2}+\beta_{lh}r\right)\left(2
\beta_{lf}\beta_2-\theta^2\right)}{I\beta_{lh}\left(4\beta_{lf}\beta_g-
\theta^2\right)+\beta_{lf}\left(4\beta_{lf}\beta_g-2\theta^2\right)} \tag*{$(5.19)$}
\end{equation*}

\begin{equation*}
Q^\ast_g=\frac{\beta_g\left(I\beta_{lh}\theta\left(\alpha_{lf}+\theta
C_g\right)+2\beta_{lf}\left(\alpha_g-\beta_gC_g\right)\left(I\beta_{lh}
\beta_{lf}+1\right)\right) + \beta_g\beta_{lf}\theta\left(\alpha_{lh}+2\alpha_{lf}-2K_{l2}+2\theta
C_g+\beta_{lh}r\right)}{I\beta_{lh}\left(4\beta_{lf}\beta_g-\theta^2
\right)+\beta_{lf}\left(4\beta_{lf}\beta_g-2\theta^2\right)} \tag*{$\left(5.20\right)$}
\end{equation*}

Substituting $P^{\ast\text{+}}_g$ in (4.16), we get
\begin{equation*}
\lambda_{l2}=\frac{I\left(2\beta_{lf}\beta_g\left(2\alpha_{lh}+2
\alpha_{lf}-4K_{l2}+\theta
C_g-2\beta_{lh}C_l\right)+2\theta\beta_{lf}\alpha_g\right) + I\theta^2\left(-\alpha_{lh}+2K_{l2}+\beta_{lh}C_l\right)-2\beta_{lf}
\left(C_l+r\right)\left(2\beta_{lf}\beta_g-\theta^2\right)}{I\beta_{lh}
\left(4\beta_{lf}\beta_g-\theta^2\right)+\beta_{lf}\left(4\beta_{lf}\beta_g-2
\theta^2\right)} \tag*{$\left(5.21\right)$}
\end{equation*}

Hence, if we assume that demand base and consumer price sensitivity are the same for both manufacturers at the foreign market, then the optimal prices and quantities can be written as:

\begin{equation*}
P^{\ast^{-}}_{lh2}=\frac{I\beta^2\left(4\alpha_{lh}+4\alpha-8K_{l2}+2\theta
C_g-4C_l\beta_{_{lh}}\right) - I\left(\theta^2\left(\alpha_{_{lh}}-K_{l2}\right)-\theta\beta\alpha
\right)  }{(\beta+I\beta_{lh})\left(4\beta^2-\theta^2
\right)}
\end{equation*}
\begin{equation*}
+\frac{\beta\left(4\beta^2\left(\alpha_{_{lh}}-\beta_{_{lh}}C_l\right)-%
\theta^2\left(\alpha_{_{lh}}-\beta_{_{lh}}\left(C_l+r\right)\right)\right)}{2%
\beta_{_{lh2}}(\beta+I\beta_{_{lh}})\left(4\beta^2-\theta^2\right)}
\end{equation*}

\begin{equation*}
P^{\ast^{-}}_{lf2}=\frac{I\left(\beta_{_{lh}}\left(2\beta\alpha+\theta\alpha+%
\theta\beta
C_g\right)+2\beta^2\alpha_{_{lh}}\right) + 2\beta^2\left(2\alpha-2K_{l2}+\theta
C_g+\beta_{_{lh}}r\right)}{4\beta^2(\beta+I\beta_{_{lh}})}
\end{equation*}
\begin{equation*}
-\frac{\theta^2\left(\alpha_{_{lh}}-2K_{l2}-C_l\beta_{_{lh}}\right)+4\theta
\beta\alpha}{2(\beta+I\beta_{_{lh}})\left(4\beta^2-\theta^2\right)} + \frac{\theta^2\left(C_l+r\right)}{I(\beta+I(t)\beta_{_{lh}})\left(4\beta^2-
\theta^2\right)}
\end{equation*}

%\begin{equation*}
%\frac{\theta^2\left(C_l+r\right)}{I(\beta+I(t)\beta_{_{lh}})\left(4\beta^2-%
%\theta^2\right)}
%\end{equation*}

\begin{equation*}
P^{\ast^{-}}_g=\frac{I\beta_{lh}\left(2\beta\left(\alpha+\beta
C_g\right)+\theta\alpha\right) + \beta_{lf}\left(\left(2\beta\left(\alpha+\beta
C_g\right)+\theta\alpha_{lf}\right)+\theta\left(\alpha_{lh}+2\alpha-2K_{l2}+
\beta_{lh}r\right)\right)}{I\beta_{lh}\left(4\beta^2-\theta^2\right)+
\beta\left(4\beta^2-2\theta^2\right)}
\end{equation*}

Thus, 
\begin{equation*}
Q^{\ast^{-}}_{lh2}=\frac{2 I\beta_{_{lh}}\left( \beta^2
\left(4K_{l2}-2\alpha-\theta C_g\right)-\theta\left(\beta\alpha+\theta
K_{l2}\right)\right) + \beta\left(4\beta^2\left(\alpha_{_{lh}}+\beta_{_{lh}}r\right)-\theta^2
\beta\left(\alpha_{_{lh}}+\beta_{_{lh}}\left(C_l+2r\right)\right)\right) }{ 2(\beta+I\beta_{_{lh}})\left(4\beta^2-\theta^2\right)}
\end{equation*}

\begin{equation*}
Q^{\ast^{-}}_{lf2}=\frac{2 I \beta\beta_{_{lh}}\left(2\alpha\left(2\beta+\theta
\right)+\theta\beta
C_g\right) + \beta\left(4\beta^2\left(2K_{l2}-\alpha_{_{lh}}-\beta_{_{lh}}r\right)+
\theta^2\left(\alpha_{_{lh}}-2K_{l2}+\beta_{_{lh}}\left(C_l+r\right)\right)
\right)}{2 (\beta+I\beta_{_{lh}})\left(4\beta^2-\theta^2\right)} 
\end{equation*}

%\begin{equation*}
%\frac{\beta\left(4\beta^2\left(2K_{l2}-\alpha_{_{lh}}-\beta_{_{lh}}r\right)+
%\theta^2\left(\alpha_{_{lh}}-2K_{l2}+\beta_{_{lh}}\left(C_l+r\right)\right)
%\right)}{2(\beta+I\beta_{_{lh}})\left(4\beta^2-\theta^2\right)}
%\end{equation*}

\begin{equation*}
Q^\ast_g=\frac{\beta\left(I\beta_{lh}\theta\left(\alpha+\theta
C_g\right)+2\beta\left(\alpha-\beta
C_g\right)\left(I\beta_{lh}\beta+1\right)\right) + \beta^2\theta\left(\alpha_{lh}+2\alpha-2K_{l2}+2\theta
C_g+\beta_{lh}r\right)}{I\beta_{lh}\left(4\beta^2-
\theta^2\right)+\beta_{lf}\left(4\beta^2-2\theta^2\right)}
\end{equation*}
\\

\noindent \textbf{Proof of Colloary 1} 
From equations (\ref{entrant price incumbent un}) $ P^{u}_{ei}(P^{u}_{ii}) $  and \ref{incumbent price un}  $P^{u}_{ii} (P^{u}_{ei})$, we can get the incumbent's optimal quantity as: 
\begin{equation*}
{Q_i^{u}}^{*} = \frac{\beta_{ii} \left(A \right)}{I \left(4 \beta_{ei} \beta_{ii}-\theta^2\right)} \ ,
\end{equation*}
where $A =\beta_{ii} \left(\beta_{ei} \theta  (C_{e}+s) - C_{i} I (2  \beta_{ei} \beta_{ii} - \theta^2)+ \alpha_{i} I (2 \beta_{ei} \phi +\theta  (1-\phi) )\right) > 0$. 
\begin{equation*}
{\Pi_i^{u}}^{*} = \frac{\beta_{ii} \left(A\right)^{2}}{I^2 \left(4 \beta_{ei} \beta_{ii} - \theta^2 \right)^2 } \ .
\end{equation*}
Take the first derivative with regarding to $I$, we can get
\begin{equation*}
{{\Pi_i^{u}}^{*}}^{'} = - \frac{2 (C_{e}+s) \beta_{ei} \beta_{ii} \left( A \right)}{I^3 \left(4 \beta_{ei} \beta_{ii} - \theta^2 \right)^2 }  < 0\ .
\end{equation*}

\noindent \textbf{Proof of Lemma 4.5} 

It directly follows from that when $\alpha_{e} >  \frac{\alpha_i (2(1-\phi) + \theta \phi) + C_{i} \theta }{4 - \theta ^2} +C_e $ then $K_Q > K_{h}$

\noindent \textbf{Proof of Lemma 4.6} 

\noindent Proof $ I_h - I_t > 0 $ . 

\begin{equation*}
I_{h} (K) = \frac{\left(2- \theta ^2 \right) (\alpha_e + s)}{\alpha_i (2- (2- \theta) \phi) + C_{i} \theta - \left(4 - \theta ^2 \right) K}
\end{equation*}
\begin{equation*}
I_t (K) = \frac{2 \left(2- \theta ^2 \right) (C_e + s)}{2 \alpha_{i}(2- (2- \theta) \phi)  + (\alpha_{e} -  C_i - 2 K) \left(4 - \theta ^2\right)+2 C_{i} \theta}
\end{equation*}
Let $A = \alpha_i (2- (2- \theta) \phi) + C_{i} \theta - \left(4 - \theta ^2 \right) K $  and Let $ B =2 \alpha_{i}(2- (2- \theta) \phi)  + (\alpha_{e} -  C_i - 2 K) \left(4 - \theta ^2\right)+2 C_{i} \theta $, it can be shown that $B - 2A = (4 - \theta ^2) (\alpha_e - C_e) > 0 $.  And in the numerator,  $\alpha_e > C_e$, thus $\alpha_e + s > C_e + s $. Therefore, we can get $ I_h > I_t $.  \\

\noindent Proof $ I_h - I_f > 0 $  \\
We know that
\begin{equation*}
I_f (K)= \frac{\left(2-\theta ^2\right) (\alpha_{e}  + s - 2 k)}{\alpha_i (2- (2- \theta) \phi) + C_{i} \theta} \ ,
\end{equation*}
and $I_{f}(K)$ is an decreasing function of $K$ and $I_{h}(K)$ is an increasing function of $K$. It can be shown that $I_{f}(0) = I_{h}(0)  $ thus  $ I_h > I_f  $.  \\

\noindent Proof $ I_t - I_z > 0 $  \\
\begin{equation*}
I_z = \frac{\left(2-\theta ^2\right) (C_e + s)}{\alpha_i (2- (2- \theta) \phi) + C_{i} \theta }
\end{equation*}
Substitute $K_Q$ into $I_t (K)$ and we can get $I_t (K_Q) = I_z$. And $I_t(k)$ is an increasing function of $k$, therefore $I_t \geq I_z$ on $[K_Q, +\infty)$. \\

\noindent Proof $ K_t  >  K_h $  \\
\begin{equation*}
K_t =\frac{2 \alpha_{i}(2- (2- \theta) \phi)  + (\alpha_{e} -  C_i) \left(4 - \theta ^2\right)+2 C_{i} \theta }{8-2 \theta ^2}
\end{equation*}
\begin{equation*}
K_h = \frac{\alpha_i (2- (2- \theta) \phi) + C_{i} \theta  }{4 - \theta ^2}
\end{equation*}
$K_t - K_h = \frac{\alpha_e - C_e}{2} > 0$. 

$K_t - K_Q = \frac{\alpha_i (2- (2- \theta) \phi) + C_{i} \theta }{4 - \theta ^2} > 0$.
